# Supplementary material for: Request-and-Reverify: Hierarchical Hypothesis Testing for Concept Drift Detection with Expensive Labels
Source: arXiv:1806.10131 ancillary file (2018-06-28)
Supplement: Supplementary file 1 [file SupplementaryMaterial_IJCAI-18.pdf]

# Request-and-Reverify: Hierarchical Hypothesis Testing for Concept Drift Detection with Expensive Labels - Supplementary Material

Shujian Yu[1,2], Xiaoyang Wang[1], José C. Príncipe[2]
[1] Nokia Bell Labs, Murray Hill, NJ, USA, [2] University of Florida, Gainesville, FL, USA
yusjlcy9011@ufl.edu, xiaoyang.wang@nokia-bell-labs.com, principe@cnel.ufl.edu

This supplementary material contains additional experimental results of our proposed approaches described in the IJCAI-18 paper [1] entitled "Request-and-Reverify: Hierarchical Hypothesis Testing for Concept Drift Detection with Expensive Labels."

## I. Experiments on benchmark synthetic data

TABLE I

Averaged Normalized Area Under the Curve (NAUC) values for Precision-Range curve (left side of the forward slash) and Recall-Range curve (right side of the forward slash) of all competing algorithms using $k$-nearest neigobors (KNN) classifier. The performance of MD3 and CDBD is omitted because they are SVM-specific. The best three results are marked with red, blue and green respectively. "-" denotes no concept drift is detected.

| | **Our methods** | | **Unsupervised methods** | **Supervised methods** | | | | |
|---|---|---|---|---|---|---|---|---|
| | HHT-CU | HHT-AG | A-KS | HLFR | LFR | DDM | EDDM | HDDM |
| 2CDT | 0.89 / 0.89 | 0.20 / 0.76 | 0.18 / 0.60 | 0.94 / 0.71 | 0.94 / 0.71 | 0.79 / 0.79 | 0.75 / 0.75 | 0.90 / 0.90 |
| 2CHT | 0.89 / 0.89 | 0.19 / 0.76 | 0.18 / 0.59 | 0.95 / 0.95 | 0.95 / 0.95 | 0.29 / 0.29 | 0.66 / 0.66 | 0.83 / 0.83 |
| UG-2C-2D | 0.64 / 0.64 | 0.17 / 0.14 | 0.09 / 0.16 | 0.52 / 0.40 | 0.47 / 0.54 | 0.40 / 0.63 | 0.55 / 0.78 | 0.62 / 0.62 |
| MG-2C-2D | 0.34 / 0.68 | 0.29 / 0.38 | 0.26 / 0.60 | 0.52 / 0.91 | 0.38 / 0.91 | 0.32 / 0.72 | 0.24 / 0.72 | 0.21 / 0.49 |
| 4CR | - / 0 | - / 0 | - / 0 | | | 0.53 / 0.89 | 0.86 / 0.86 | 0.99 / 0.99 |
| 4CRE-V1 | 0.94 / 0.94 | 0.07 / 0.07 | 0.06 / 0.06 | | | 0.08 / 0.10 | 0.67 / 0.84 | 0.99 / 0.99 |
| 4CR1CF | 0.73 / 0.80 | 0.12 / 0.06 | 0.06 / 0.03 | | | 0.53 / 0.89 | 0.45 / 0.90 | 0.36 / 0.72 |
| 5CVT | 0.41 / 0.94 | 0.18 / 0.66 | 0.17 / 0.80 | | | 0.41 / 0.67 | 0.18 / 0.47 | 0.37 / 0.71 |

TABLE II

Averaged Normalized Area Under the Curve (NAUC) values for Precision-Range curve (left side of the forward slash) and Recall-Range curve (right side of the forward slash) of all competing algorithms using naive Bayes (NB) classifier. The performance of MD3 and CDBD is omitted because they are SVM-specific. The best three results are marked with red, blue and green respectively. "-" denotes no concept drift is detected.

| | **Our methods** | | **Unsupervised methods** | **Supervised methods** | | | | |
|---|---|---|---|---|---|---|---|---|
| | HHT-CU | HHT-AG | A-KS | HLFR | LFR | DDM | EDDM | HDDM |
| 2CDT | 0.56 / 0.61 | 0.20 / 0.77 | 0.18 / 0.53 | 0.78 / 0.74 | 0.78 / 0.66 | 0.77 / 0.71 | 0.73 / 0.73 | 0.87 / 0.87 |
| 2CHT | 0.60 / 0.51 | 0.19 / 0.79 | 0.18 / 0.76 | 0.96 / 0.96 | 0.91 / 0.84 | 0.44 / 0.44 | 0.87 / 0.87 | 0.80 / 0.80 |
| UG-2C-2D | 0.59 / 0.59 | 0.29 / 0.58 | 0.26 / 0.59 | 0.76 / 0.96 | 0.76 / 0.96 | 0.23 / 0.61 | 0.51 / 0.64 | 0.71 / 0.71 |
| MG-2C-2D | 0.50 / 0.72 | 0.17 / 0.14 | 0.11 / 0.07 | 0.77 / 0.96 | 0.77 / 0.96 | 0.28 / 0.42 | 0.27 / 0.88 | 0.86 / 0.86 |
| 4CR | - / 0 | - / 0 | - / 0 | | | 0.95 / 0.96 | 0.86 / 0.86 | 0.99 / 0.99 |
| 4CRE-V1 | 0.83 / 0.61 | 0.37 / 0.31 | 0.34 / 0.34 | | | 0.13 / 0.17 | 0.82 / 0.82 | 0.98 / 0.98 |
| 4CR1CF | 0.39 / 0.31 | 0.34 / 0.15 | 0.17 / 0.09 | | | 0.79 / 0.86 | 0.28 / 0.54 | 0.96 / 0.96 |
| 5CVT | 0.24 / 0.26 | 0.19 / 0.77 | 0.17 / 0.87 | | | 0.49 / 0.78 | 0.21 / 0.60 | 0.77 / 0.79 |

TABLE III

Averaged number of required labeled samples (%) for all competing algorithms using $k$-nearest neigobors (KNN) classifier and naive Bayes (NB) classifier. The performance of HLFR, LFR and DDM is omitted because they require all the true labels (i.e., 100%). The performance of MD3 and CDBD is also omitted because they are SVM-specific. "**0**" means that no concept drift is detected.

| | **HHT-CU** | | **HHT-AG** | | **A-KS** | |
|---|---|---|---|---|---|---|
| | KNN | NB | KNN | NB | KNN | NB |
| 2CDT | **34.67** | **34.33** | 97.38 | 97.71 | 73.08 | 74.22 |
| 2CHT | **44.45** | **38.19** | 96.47 | 96.44 | 74.36 | 74.36 |
| UG-2C-2D | 37.48 | 28.09 | 37.13 | 38.93 | **13.64** | **13.33** |
| MG-2C-2D | 32.98 | 22.48 | 30.02 | 30.57 | **13.66** | **13.33** |
| 4CR | 0 | 0 | 0 | 0 | 0 | 0 |
| 4CRE-V1 | 22.92 | 21.46 | 32.55 | 35.11 | **15.83** | **16.38** |
| 4CR1CF | 27.84 | 27.42 | 22.91 | 24.97 | **8.33** | **8.33** |
| 5CVT | **32.46** | **36.14** | 38.79 | 38.76 | 43.88 | 43.88 |

TABLE IV

SUMMARY OF $p$-VALUES AND DECISION VALUES (IN PARENTHESES) USING WILCOXON RANK-SUM TEST AT 0.1 SIGNIFICANCE LEVEL ON THE RANK OF (A) **PRECISION-RANGE** NAUC VALUES AND (B) **RECALL-RANGE** NAUC VALUES BETWEEN OUR METHODS AND ALL COMPETING METHODS. THE VALUE UNDER EACH METHOD INDICATES THE AVERAGE RANK. SOFT MARGIN SVM IS SELECTED AS THE BASELINE CLASSIFIER.

(a) Precision-Range NAUC values statistical comparison

| | **HHT-CU** (2.71) | **HHT-AG** (5.57) | A-KS (6.57) | MD3 (9.75) | CDBD (9.25) | HLFR (1.75) | LFR (3.25) | DDM (4.13) | EDDM (4.00) | HDDM (1.75) |
|---|---|---|---|---|---|---|---|---|---|---|
| **HHT-CU** | - | 0.018 (1) | 0.002 (1) | 0.029 (1) | 0.029 (1) | 0.400 (0) | 0.571 (0) | 0.015 (1) | 0.066 (1) | 0.251 (0) |
| **HHT-AG** | 0.018 (1) | - | 0.275 (0) | 0.029 (1) | 0.029 (1) | 0.029 (1) | 0.029 (1) | 0.363 (0) | 0.212 (0) | 0.004 (1) |

(b) Recall-Range NAUC values statistical comparison

| | **HHT-CU** (4.14) | **HHT-AG** (6.14) | A-KS (6.71) | MD3 (9.75) | CDBD (2.25) | HLFR (4.00) | LFR (2.00) | DDM (4.50) | EDDM (4.25) | HDDM (2.75) |
|---|---|---|---|---|---|---|---|---|---|---|
| **HHT-CU** | - | 0.212 (0) | 0.080 (1) | 0.029 (1) | 0.026 (1) | 0.858 (0) | 0.200 (0) | 0.514 (0) | 0.835 (0) | 0.330 (0) |
| **HHT-AG** | 0.212 (0) | - | 0.839 (0) | 0.086 (1) | 0.029 (1) | 0.029 (1) | 0.029 (1) | 0.361 (0) | 0.265 (0) | 0.066 (1) |

TABLE V

SUMMARY OF $p$-VALUES AND DECISION VALUES (IN PARENTHESES) USING WILCOXON RANK-SUM TEST AT 0.1 SIGNIFICANCE LEVEL ON THE RANK OF (A) **PRECISION-RANGE** NAUC VALUES AND (B) **RECALL-RANGE** NAUC VALUES BETWEEN OUR METHODS AND ALL COMPETING METHODS. THE VALUE UNDER EACH METHOD INDICATES THE AVERAGE RANK. NEAREST NEIGHBORS (NN) IS SELECTED AS THE BASELINE CLASSIFIER.

(a) Precision-Range NAUC values statistical comparison

| | **HHT-CU** (2.14) | **HHT-AG** (5.71) | A-KS (6.86) | HLFR (1.75) | LFR (2.25) | DDM (3.88) | EDDM (4.13) | HDDM (3.25) |
|---|---|---|---|---|---|---|---|---|
| **HHT-CU** | - | 0.001 (1) | 0.001 (1) | 0.486 (0) | 0.571 (0) | 0.068 (1) | 0.020 (1) | 0.224 (0) |
| **HHT-AG** | 0.001 (1) | - | 0.140 (0) | 0.029 (1) | 0.057 (1) | 0.108 (0) | 0.145 (0) | 0.025 (1) |

(b) Recall-Range NAUC values statistical comparison

| | **HHT-CU** (2.57) | **HHT-AG** (5.71) | A-KS (6.00) | HLFR (3.50) | LFR (3.25) | DDM (3.63) | EDDM (3.50) | HDDM (3.13) |
|---|---|---|---|---|---|---|---|---|
| **HHT-CU** | - | 0.004 (1) | 0.008 (1) | 1.000 (0) | 0.886 (0) | 0.137 (0) | 0.396 (0) | 0.425 (0) |
| **HHT-AG** | 0.004 (1) | - | 0.441 (0) | 0.343 (0) | 0.286 (0) | 0.030 (1) | 0.160 (0) | 0.015 (1) |

TABLE VI

SUMMARY OF $p$-VALUES AND DECISION VALUES (IN PARENTHESES) USING WILCOXON RANK-SUM TEST AT 0.1 SIGNIFICANCE LEVEL ON THE RANK OF (A) **PRECISION-RANGE** NAUC VALUES AND (B) **RECALL-RANGE** NAUC VALUES BETWEEN OUR METHODS AND ALL COMPETING METHODS. THE VALUE UNDER EACH METHOD INDICATES THE AVERAGE RANK. NAIVE BAYES (NB) IS SELECTED AS THE BASELINE CLASSIFIER.

(a) Precision-Range NAUC values statistical comparison

| | **HHT-CU** (3.86) | **HHT-AG** (5.71) | A-KS (6.86) | HLFR (1.50) | LFR (1.75) | DDM (4.38) | EDDM (4.25) | HDDM (1.63) |
|---|---|---|---|---|---|---|---|---|
| **HHT-CU** | - | 0.040 (1) | 0.004 (1) | 0.029 (1) | 0.029 (1) | 0.533 (0) | 0.470 (0) | 0.020 (1) |
| **HHT-AG** | 0.040 (1) | - | 0.164 (0) | 0.029 (1) | 0.029 (1) | 0.354 (0) | 0.124 (0) | 0.002 (1) |

(b) Recall-Range NAUC values statistical comparison

| | **HHT-CU** (5.43) | **HHT-AG** (5.14) | A-KS (5.57) | HLFR (1.50) | LFR (2.75) | DDM (4.63) | EDDM (3.25) | HDDM (2.13) |
|---|---|---|---|---|---|---|---|---|
| **HHT-CU** | - | 0.770 (0) | 0.727 (0) | 0.029 (1) | 0.086 (1) | 0.660 (0) | 0.023 (1) | 0.006 (1) |
| **HHT-AG** | 0.770 (0) | - | 0.558 (0) | 0.058 (1) | 0.171 (0) | 0.981 (0) | 0.059 (1) | 0.009 (1) |

To explain the statistic analysis results in Table IV, Table V, and Table VI, we take HHT-CU in Table IV(a) as an example. 1) Comparing HHT-CU with HDDM, although their ranks differ (HHT-CU ranks 2.71, whereas HDDM ranks 1.75), the Wilcoxon rank-sum test outputs a $p$-value of 0.251. Therefore, the rank difference between HHT-CU and HDDM under 0.1 significance level is not statistically significant, i.e., these two methods perform similarly. 2) Comparing HHT-CU with DDM, their ranks differ as well (HHT-CU ranks 2.71, whereas DDM ranks lower at 4.13). However, the Wilcoxon rank-sum test outputs a $p$-value of 0.015. Therefore, the rank difference between HHT-CU and DDM under 0.1 significance level is statistically significant, i.e., HHT-CU outperforms DDM.

In most of the cases, the precision values of HHT-CU are significant higher than those of its unsupervised counterparts (i.e., MD3, CDBD and A-KS) and of the popular concept drift detectors (e.g., DDM and EDDM). Although HDDM or HLFR seem to have higher precision than HHT-CU, the difference is small. Since the precision value is directly associated with false positive rate, the statistic analysis results further validate the effectiveness of HHT framework on rejecting false detections, thus reducing the Type-I error. On the other hand, it is interesting to find that, in most of the cases, the recall values of HHT-CU are

not significantly different from its supervised counterparts, including DDM, EDDM, LFR, HLFR and HDDM. This suggests that all these methods have statistically similar detection powers. As a result, their possibilities of Type-II errors are close.

## II. Results on real-world data using nearest neigobors and naive Bayes

The concept drift detection results and streaming data classification results on real-world data using Nearest Neighbors (NN) classifier and Naive Bayes (NB) classifier are summarized in Table VII and Table VIII respectively. In most of the cases, the HHT-CU can achieve satisfying or even the best overall performance in terms of accurate drift detection, streaming classification, as well as the efficient utilization of labeled data.

TABLE VII
Quantitative metrics on real-world applications using Nearest Neighbors (NN) classifier. The **Precision**, **Recall** and **Delay** denote the concept drift detection precision values, recall values and detection of delay, where the **Accuracy** and **Labels** denotes the (overall) cumulative classification accuracy and required portion of true labels (%). The best result is marked with red. "-" denotes no concept drift is detected.

| | **USENET1** | | | | | **Keystroke** | | | | | **Posture** | | | | |
|---|---|---|---|---|---|---|---|---|---|---|---|---|---|---|---|
| | Precision | Recall | Delay | Accuracy | Labels | Precision | Recall | Delay | Accuracy | Labels | Precision | Recall | Delay | Accuracy | Labels |
| HHT-CU | 1.00 | 1.00 | 5.5 | 84 | 84.67 | 1.00 | 0.43 | 2.33 | 94 | 42.86 | 0.57 | 1.00 | 1404 | 67 | 10.12 |
| HHT-AG | - | 0 | - | 55 | 0 | 0.5 | 0.14 | 1 | 80 | 57.70 | 0.25 | 0.5 | 87 | 63 | 17.97 |
| A-KS | - | 0 | - | 55 | 0 | 0.25 | 0.14 | 1 | 83 | 52.43 | 0.25 | 0.5 | 87 | 63 | 10.54 |
| HLFR | 0.4 | 0.5 | 8.5 | 83 | 100 | | | | | | | | | | |
| LFR | 0.33 | 0.5 | 8.5 | 83 | 100 | | | | | | | | | | |
| DDM | 0.33 | 0.5 | 15.5 | 82 | 100 | - | 0 | - | 88 | 100 | 1.00 | 0.25 | 682 | 44 | 100 |
| EDDM | 0.75 | 0.75 | 39.3 | 81 | 100 | 0.67 | 0.29 | 30.5 | 81 | 100 | 0.50 | 0.50 | 2805.5 | 57 | 100 |
| HDDM | 1.00 | 1.00 | 11.25 | 82 | 100 | 1.00 | 0.14 | 4 | 89 | 100 | 0.57 | 1.00 | 1445.8 | 65 | 100 |

TABLE VIII
Quantitative metrics on real-world applications using Naive Bayes (NB) classifier. The **Precision**, **Recall** and **Delay** denote the concept drift detection precision values, recall values and detection of delay, where the **Accuracy** and **Labels** denotes the (overall) cumulative classification accuracy and required portion of true labels (%). The best result is marked with red. "-" denotes no concept drift is detected.

| | **USENET1** | | | | | **Keystroke** | | | | | **Posture** | | | | |
|---|---|---|---|---|---|---|---|---|---|---|---|---|---|---|---|
| | Precision | Recall | Delay | Accuracy | Labels | Precision | Recall | Delay | Accuracy | Labels | Precision | Recall | Delay | Accuracy | Labels |
| HHT-CU | 0.6 | 0.75 | 16.67 | 82 | 71.54 | 0.5 | 0.14 | 1 | 82 | 28.57 | 1.00 | 1.00 | 2405.33 | 46 | 14.83 |
| HHT-AG | - | 0 | - | 55 | 0 | 0.5 | 0.14 | 1 | 75 | 57.11 | 0.29 | 0.5 | 81.5 | 45 | 18.05 |
| A-KS | - | 0 | - | 55 | 0 | 0.25 | 0.14 | 1 | 75 | 52.43 | 0.25 | 0.5 | 159.5 | 45 | 10.54 |
| HLFR | 1.00 | 1.00 | 8.5 | 85 | 100 | | | | | | | | | | |
| LFR | 1.00 | 1.00 | 8.5 | 85 | 100 | | | | | | | | | | |
| DDM | 0.75 | 0.75 | 17.33 | 82 | 100 | 0.2 | 0.14 | 10 | 84 | 100 | 0.75 | 0.75 | 3987.33 | 45 | 100 |
| EDDM | 0.75 | 0.75 | 47 | 82 | 100 | 0.33 | 0.14 | 4 | 75 | 100 | 0.75 | 0.75 | 1988.8 | 45 | 100 |
| HDDM | 1.00 | 1.00 | 17.25 | 83 | 100 | - | 0 | - | 69 | 100 | 1.00 | 1.00 | 1445.8 | 46 | 100 |

## III. Comparison with active learning [2]

It is worth noting that, although both HHT-CU and the active learning method in [2] both request labels when certain conditions are met, their mechanisms are totally different. The active learning strategy [2] explicitly assigns a hard ratio as the budget limit. If budget permits, the algorithm would request labels once the threshold criterion is met; otherwise, it would reject labeling requests. By contrast, HHT-CU does not incorporate any budget limits. By this, the number of labels requested depends largely on the significance level of Layer-I test: a large significance level in Layer-I will cause more potential drift points, thus increasing the number of requested labels for validation in Layer-II. On the other hand, a small significance level would decrease the number of labels requested. Moreover, in extremely low significance level (e.g., 0.001), the Layer-I test of HHT-CU is prone to miss the true drifting points, and thus the accuracy is lower than those of higher significance levels (e.g. 0.01). As a result, the Table 1 of our paper [1] recommends $\Theta_1 = 0.01$ by default.

From Fig. 1, we can see the accuracy of HHT-CU is not sensitive to the significance level once the significance level is large enough. Comparatively, the performances of active learning methods in [2] obviously decrease once the budget level gradually becomes smaller. More importantly, the HHT-CU in most cases outperforms the active learning methods in [2]. At the 30% budget level, it outperforms the active learning methods by approximately 10% in the absolute value.

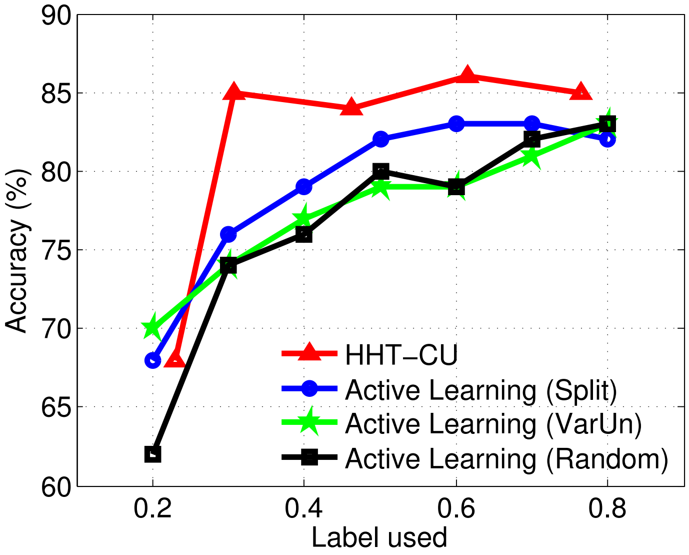


Fig. 1. Classification accuracy comparison between HHT-CU and active learning methods in [2] on USENET1 dataset given different number of labels. Three active learning strategies are selected for comparison: 1) split strategy, 2) variable uncertainty strategy, and 3) random strategy. For HHT-CU, the number of required labels is determined by the significance level $\Theta_1$ of Layer-I test. We select five different values of $\Theta_1$: 0.001, 0.01, 0.05, 0.1 and 0.2, the used label ratios are 0.2308, 0.3077, 0.4615, 0.6154 and 0.7654 respectively, and the corresponding classification accuracies are 68, 85, 84, 86, and 85 respectively. SVM is selected as the baseline classifier.

## References

[1] S. Yu, X. Wang, and J. C. Príncipe, "Request-and-reverify: Hierarchical hypothesis testing for concept drift detection with expensive labels," in *27th International Joint Conference on Artificial Intelligence*, 2018.

[2] I. Žliobaite, A. Bifet, B. Pfahringer, and G. Holmes, "Active learning with drifting streaming data," *IEEE Trans. Neural Netw. Learn. Syst.*, vol. 25, no. 1, pp. 27–39, 2014.
